# Supplementary material for: Individual Fairness for $k$-Clustering
Source: arXiv:2002.06742 source file (2020-09-21)
Supplement: Supplementary file 1 [file appendix.tex]

\section{Miscellaneous}

\begin{theorem}[$(O(\log n), O(1))$-approximation for $\alpha$-Fair $k$-Median Clustering]
For any $\alpha\geq 2$, there exists a $(O(\log n), O(1))$-approximation algorithm for the $\alpha$-fair $k$-Median problem in a $d$-dimensional Euclidean space that runs in $\poly(n)\cdot 2^{O(dk)}$.\footnote{We remark that the algorithms satisfies the ``cost guarantee'' on expectation; i.e., $\E[\cost(\sol)] \leq \log n \cdot \cost(\opt_{\alpha})$.}
\end{theorem}
\begin{proof}
First we embed the given set of points $P \in \mathbb{R}^d$ into a tree metric called $\gamma$-HST with $\gamma=O(1)$. This parts mainly contributes to the expected $\log n$ bound for the ``cost guarantee''; this is a {\em non-contracting} embedding with {\em expected} distortion of $O(\log n)$. 

Next, we find an optimal $O(\alpha)$-fair solution of the embedded instance with respect to the $k$-Median cost function using a dynamic programming approach. Note that the naive approach will have $2^n$ dependence in the runtime because there are $n$ constraints (one for the fairness guarantee of each point). Moreover, we cannot naively use the tree information to determine the $n/k$ neighborhood of the points because the only guarantee that we have is on expectation.

Here is our approach to reduce the dependence of $2^n$ to $2^k$. This is by the second property in Observation~\ref{obsr:MM}. Basically, it suffices to make sure that fairness guarantee is satisfied for the center points returned by the greedy algorithm of~\cite{charikar2010local}. Then, for all points in $P$, the resulting clustering will be $(\alpha+2)$-fair.   
\end{proof}

\subsection{Improving the $2^k$ Dependence in the Runtime.}
{\bf High-level Approach.} Here is the high-level description of our approach to reduce the exponential dependence on $k$ down to $\poly(k)$. Consider an optimal $\alpha$-fair $k$-median clustering of $P$ and denote its centers by $S_{\opt}$.
\begin{enumerate}
\item First, we show that each center $c\in S$ has $O({n\over k})$ ``alternatives'' that can replace $c$ without violating any of {\it cost} and {\it fairness}\footnote{For Makarychevs' centers} guarantees of $\alpha$-fairness $k$-median clustering.
\item Next, we show in an embedding of $P$ into $\gamma$-HST, with high probability, the distances of all Makarychevs' centers to at least one of their alternatives are preserved up to a $\log n$ factor.\footnote{Most likely up to a constant factor with a more careful analysis.} In other words, for each center of interest, there is an alternative point in distance at most $O(r_{k} \cdot \log n)$.
\item Finally, we can instead keep track of the {\it fairness} guarantee implicitly via a modified dynamic programming approach on the tree representation of $P$. Hence, the dependence on $k$ reduces to $\poly(k)$. 
\end{enumerate}

\begin{remark}
To show step $1$ in the above description is crucial that the set of points assigned to each Makarychevs center are disjoint. To achieve this, we modify their algorithm slightly and each time we for the selected Makarychev center $c$ assign all points at distance $4r_{k}(c)$ that are not already covered to $c$. Thus, we can argue that the set of points at distance at most $2r_k$ of centers are disjoint and each have at least $n/k$ points. Moreover, still it is easy to verify that satisfying $O(\alpha)$-fairness for these centers guarantees $O(\alpha)$-fairness for all points in $P$.
\end{remark}
\section{Other Observations}
\begin{observation}
For any values of $k$ and $\alpha$, there exist instances $\script{X}$ such that for any $X\in \script{X}$, the optimal cost of  $\alpha$-fair $k$-Center of $X$ is arbitrarily larger than the optimal cost of $k$-Center of $X$.   
\end{observation}
\begin{question}
What about other clustering models? E.g., $k$-Median and $k$-Means? (it should be easy to prove a similar result there.) 
\end{question}

\begin{observation}
Let $\opt_\alpha$ denote an optimal $\alpha$-fair $k$-clustering of a pointset $P$ in a metric space $X$. Then, there exists an algorithm that returns a $2k$-clustering with set of centers of size $2k$ such that $\sol$ is a $(\alpha, k)$-fair and $\cost(\sol) \leq \eta \cdot \cost(\opt_\alpha)$ where $\eta$ is the best known approximation guarantee for the standard $k$-clustering problems.  
\end{observation}
\begin{proof}
Solve the $k$-clustering and $\alpha$-fairness problems separately and combine their solutions. 
\end{proof}
